# Supplementary material for: Phase separation and multibody effects in three-dimensional active Brownian particles
Source: arXiv:2012.10365 ancillary file (2020-12-18)
Supplement: Supplementary file 1 [file supp.pdf]

# Supplementary information
# Phase separation and multibody effects in three-dimensional active Brownian particles

Francesco Turci* and Nigel B. Wilding
*H.H. Wills Physics Laboratory, Tyndall Avenue, Bristol, BS8 1TL, UK*

## S1. MODEL

Models of active Brownian particles (ABPs) have been extensively studied in the past in both two and (less often) in three dimensions (3d). Here we focus on a model of ABPs in three dimension. While in two-dimensions (2d) the freezing transition for particles interacting with repulsive central potentials is complex, and entails a fluid to hexatic and an hexatic to hexagonal transition, in 3d freezing is easier to detect as it corresponds to a single first-order phase transition. The crystalline solid is known to be face-centered cubic (fcc) and we can employ the information on this stable phase to explore coexistence at high Péclet number Pe.

Specifically, we choose to revisit the model proposed by Stenhammar et al. of repulsive active Brownian particles in three dimensions [1]. Here the particles interact exclusively via a a repulsive, short-ranged interaction provided by the truncated and shifted Weeks-Chandler-Anderson potential

$$U = 4\varepsilon\left[\left(\frac{\sigma}{r}\right)^{12} - \left(\frac{\sigma}{r}\right)^{6}\right] + \varepsilon \qquad (1)$$

with a cutoff at$r = 2^{1/6}\sigma$.

The equations of motion for the particle positions $\mathbf{r}_i$ and orientation $\mathbf{p}_i$ are:

$$\partial_{\mathrm{t}}\mathbf{r}_{\mathrm{i}} = \beta D_{\mathrm{t}}\left[\mathbf{F}_{\mathrm{i}} + F_{\mathrm{p}}\mathbf{p}_{\mathrm{i}}\right] + \sqrt{2D_{\mathrm{t}}}\mathbf{\Lambda}_{\mathrm{r}} \qquad (2)$$

$$\partial_{\mathrm{t}}\mathbf{p}_{\mathrm{i}} = \sqrt{2D_{\mathrm{r}}}\left(\mathbf{p}_{\mathrm{i}} \times \mathbf{\Lambda}_{\mathrm{p}}\right) \qquad (3)$$

The translational and rotational diffusion constants $D_{\mathrm{t}}$ and $D_{\mathrm{r}}$ coupling is $D_{\mathrm{t}} = D_{\mathrm{r}}\sigma^2/3$. The inverse thermal energy scale is set to $\beta = 1/\varepsilon$. Following Stenhammar et al. we keep the self-propulsion force constant $F_p = 24\varepsilon/\sigma$ while varying the rotational diffusion constant and hence the Péclet number $\mathrm{Pe} = v_0/(\sigma D_r)$, where $v_0 = \beta D_{\mathrm{t}} F_{\mathrm{p}}$. The terms $\mathbf{\Lambda}_{\mathrm{r}}$ and $\mathbf{\Lambda}_{\mathrm{r}}$ are unit-variance random variables with $\langle \Lambda_{\mathrm{i}}(\mathbf{r},t)\Lambda_{\mathrm{j}}(\mathbf{r}',t')\rangle = \delta_{\mathrm{ij}}\delta(\mathbf{r}-\mathbf{r}')\,\delta(t-t')$. The rotational diffusion constant defines a natural timescale for the system, the rotational diffusion time $\tau_r = 1/D_r$.

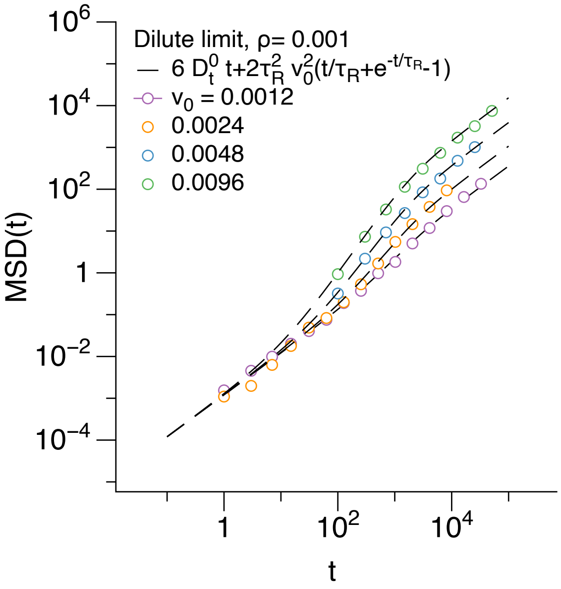


FIG. S1. Mean squared displacement of active Brownian particles in the dilute limit compared with the analytical prediction (dashed line) for several values of activity $v_0$, see Ref. [4].

To integrate the equations of motion, we implement an Euler-Maruyama scheme with constant timestep $dt = 4 \cdot 10^{-5}\tau_r$, following the Ermak–McCammon method described in detail in [2], with an in-house implementation for the molecular dynamics package LAMMPS [3]. We validate the dynamics comparing the numerically calculated mean squared displacement and the theoretical prediction in the dilute limit for different activities, see Fig. S1.

For the construction of the phase diagram, we take large systems in the slab geometry. We have considered a variety of box sizes and initial conditions.

In particular, for the gas-crystal coexistence points in Fig.1 of the manuscript, half of the system is initialised in a face-centered cubic configuration having assigned density $\rho_s$ while the rest is set to a gas density $\rho_g$. In order to avoid frustration of the crystal, the transverse box lengths $L_y = Lz$

* Corresponding author: f.turci@bristol.ac.uk

are chosen so that they can accommodate an integer number of fcc unit cells, typically 12. The longitudinal dimension is chosen to accommodate 62 of such cells. After a few steps of energy minimisation, the particle positions and orientations evolve according to the active dynamics. Depending on the system size, we run 1-3 trajectories for a total of 100-200 $\tau_r$, monitoring the stationarity of the total energy per particle. At stationarity, we compute the longitudinal density profile, fitted with

$$\rho(x) = \frac{\rho_s - \rho_g}{2} \left(\tanh[(x_0 - x)/w] + 1\right) + \rho_g, \quad (4)$$

We also tested an alternative initial condition, where the entire system is prepared in a dense crystalline state, but where the total density lower than the crystalline coexistence density. After an initial transient – which include the formation of several interfaces – only two interfaces survive and stationary gas and crystalline coexisting densities are recovered, see Fig. S2.

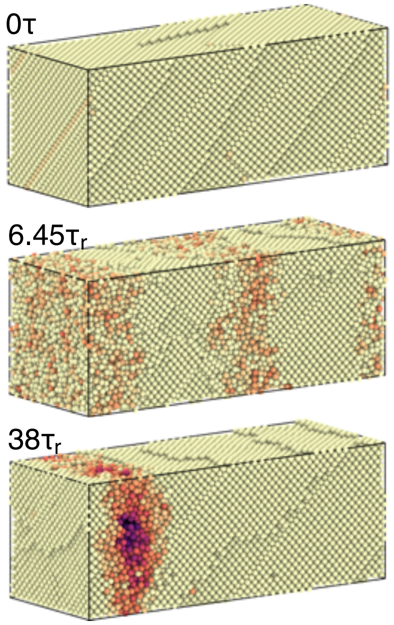


FIG. S2. Active Brownian Particles at Pe = 60 and global density $\rho = 1.34$ starting from a fully crystalline configuration in a very large system with sizes $Lx = 58.2423\sigma$ and $Ly = Lz = 22.1876\sigma$: at early stages the crystal densifies in some regions, forming multiple interfaces; however, these vanish at later stages and coexistence between a small gas region (red) and an extended crystalline region (beige) is attained.

## S2. BLOCK ANALYSIS AND COMPRESSIBILITY EQUATION

For equilibrium systems, accurate estimates of the magnitude of density fluctuations and compressibilities are normally obtained in ensembles where the number of particles can fluctuate, such as the grand canonical ensemble. This route is not available for the active system under our consideration and it is therefore necessary to resort to methods originally developed for numerical simulations in the canonical or NVT ensemble.

A previously established method is the *sub-block analysis* [5] which consists in simulating large periodic cubic boxes of linear size $L$ and sampling particle number fluctuations within extended sub-regions (blocks) of linear size $\ell = L/m$ . The procedure is sensitive to the choice of $\ell$: one chooses sub-regions that are sufficiently large to be representative of bulk fluctuations, but at the same time as numerous as possible, in order to increase the statistics and the accuracy of the estimate of the fluctuations.

In order to make a single choice of length scales across densities, we take a large cubic simulation box of linear size $L = 41.5\sigma$ and assign $m = 3, \ell = 13.83\sigma$ for the subsampling regions. In the range of number densities $[0.2, 1.3]$ this implies a total number of particles that ranges from $N = 14295$ to $N = 92915$.

The analogous of the relative compressibility is then defined as

$$\chi/\chi_{\text{ideal}} := \frac{\langle N^2 \rangle - \langle N \rangle^2}{\langle N \rangle}. \quad (5)$$

We wish to determine the maximum of $\chi/\chi_{\text{ideal}}$ with respect to variations in the density for every value of Péclet number. To do so, we evaluate the $\chi/\chi_{\text{ideal}}$ for densities in the range $[0.2, 1.2]$ with increments of $\delta\rho = 0.05$ and fit a cubic spline, from which we determine the location of the maximum. We employ $\delta\rho/2$ as an upper bound to the error in the estimate of the location of the maximum $\rho_{\chi_{\max}}$.

In equilibrium liquids the relative compressibility is given by the Ornstein-Zernicke compressibility equation

$$\frac{\chi_\infty}{\chi_\infty^{ig}} = \frac{\langle N_{\mathcal{D}}^2 \rangle - \langle N_{\mathcal{D}} \rangle^2}{\langle N_{\mathcal{D}} \rangle} = 1 + \rho \int_{\mathcal{D}} [g(\boldsymbol{r}) - 1] \mathrm{d}\boldsymbol{r}, \quad (6)$$

where $\mathcal{D}$ is the volume of a sub-region. Established originally as a mostly geometrical result by Ornstein, the connection between local fluctuations and the pair correlations expressed in the radial distribution function $g(r)$ can be derived from the properties of the grand potential of simple liquids [6].

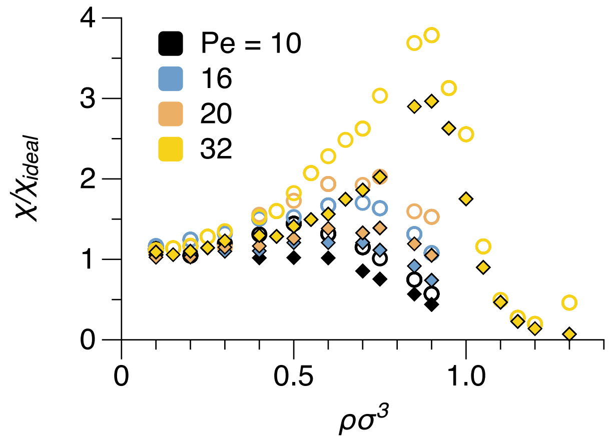


FIG. S3. Relative compressibility computed via block analysis and Eq. 5 (filled symbols) or via the radial distribution function as in Eq. 6 (empty symbols).

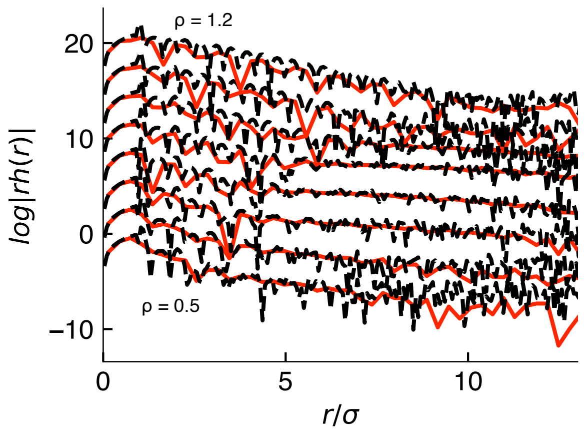


FIG. S4. Scaled total correlation functions from direct computations of the $g(r)$ (dashed lines) and from the inversion of the Fourier transform of the density-density convolution (red lines) for Pe = 28 and number densities in the interval [0.5,1.2] with increments of 0.1.

Restricting our calculations of the relative compressibility to spherical sub-domains, we can numerically test the validity of the relation in the context of dry active matter. The results in Fig. S3 underline two effects:

- the relative compressibility computed directly from the fluctuations follows the one calculated using the radial distribution function;
- there are systematic discrepancies which are greatest around the compressibility maxima.

It is known that the compressibility equation Eq. 6 holds only in a sufficiently large enough domain $\mathcal{D}$, which is also very much smaller than the box volume Hence finite size effects are likely to result in the observed discrepancies [7]. The accurate quantification of such finite-size effects and the asymptotic limit of the discrepancies is an interesting avenue of further exploration and goes beyond the scope of the present work.

## S3. CORRELATION LENGTH AND STRUCTURAL CROSSOVER

The so-called true correlation length of a liquid $\xi$ is computed from the total distribution function $h(r) = g(r) - 1$. It corresponds to the scale for the long-range exponential decay of the correlations, that can be expressed formally as

$$rh(r) \approx Ae^{-r/\xi} \tag{7}$$

The computational cost of calculating radial distribution functions increases rapidly as $N^2$. However, if we are only interested in the asymptotic decay of correlations as in Eq. 7, we can ignore the high frequency oscillations and extract the true correlation length from the spatial decay of density fluctuations. This can be done employing Fast Fourier transforms of the discretised, three-dimensional density profile, which provide the reciprocal-space correlation function, which can be finally inverse transformed to obtain $\xi$. In the discretization step, we effectively threshold the smallest lengthscale of interest, which in turn accelerates the calculation of large scale correlations for large systems of $\sim 10^5$ particles. In Fig. S4 we show that this approach allows estimation of the asymptotic, true correlation length of the system. This is possible through a linear fit of the logarithm of the total correlation function, as in Figure 2 of the main text.

In order to estimate the maximal correlation length at a given Pe, again we interpolate $\xi(\rho;\mathrm{Pe})$. We choose to identify the peak through the fitting of a Gaussian function through the data $\xi(\rho) = A + B\exp[-(\rho-\rho_{\max})^2/2\Delta^2]$ where $\Delta$ measures the width of the peak, see Fig. S5. In the phase diagram of Fig.1 in the main text, the spread $\Delta$ is represented by the shaded orange area.

A more accurate expression than Eq. 7 takes into account the presence of oscillatory behaviour in the correlations, leading to the pole formalism. For example, if two oscillatory poles are taken into consideration one can write

$$rh(r) \sim C_0 e^{-a_0 r}\cos(b_0 r - \theta_0) \tag{8}$$
$$+ C_1 e^{-a_1 r}\cos(b_1 r - \theta_1), \quad r \to \infty \tag{9}$$

with $a_0 < a_1$ defining pole 0 and pole 1 and where

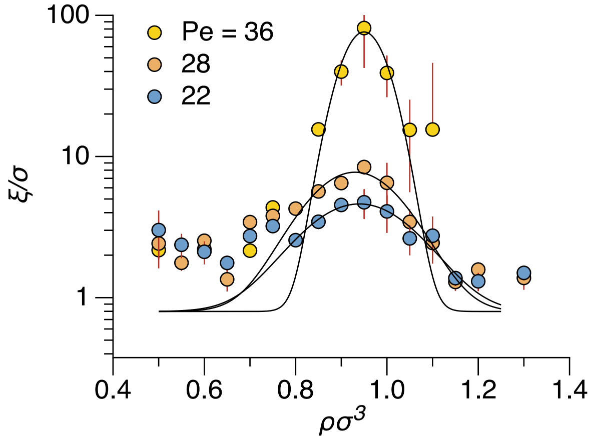


FIG. S5. Determination of the maximum correlation length: lines indicate the fit with a Gaussian function for the sole purpose of the identification of the peak location and width. The fits are restricted to densities larger than 0.6. Vertical red lines are standard errors on the lengths.

every pole contributes with its own exponential and oscillatory inverse correlation lengths $a_i = \xi_i$ and $b_i$, with amplitudes $C_i$ and phases $\theta_i$.

The increased number of parameters allows for an accurate fit of the oscillatory behaviour of the total correlation function, see Fig. S6.

Plotting the poles in a single plot for a particular Pe, see Fig. S7 reveals tha pole 0 has a non monotonic path in the $a, b$ space while pole 1 consistently picks up the monotonic increase of the short range correlation length with increasing density (as well as the narrowing of the oscillations). There is no obvious jump from one to the other pole in this plot, even if it is clear that – with increasing densities – the exponential lengthscales are approaching each other. Hence, the identification of a specific crossover point is not possible by these means.

This must be contrasted with the success of this and similar techniques and problems with equilibrium liquids, as in [8, 9]. The reason of the increased difficulty in identifying a precise crossover density can be gleaned from Fig. S6: as the density increases, the short range oscillations meet the exponentially decaying tail at larger and larger $r$. Precisions at these large $r$ requires exceedingly large simulation boxes and it is beyond the scope of the present work. Notice that, contrary to the case of simple equilibrium fluids, crossover from the exponential to the oscillatory regime is located at very high densities: this is consistent with the relatively high density of the critical point in the ABPs as opposed to relatively low number densities in equilibrium systems.

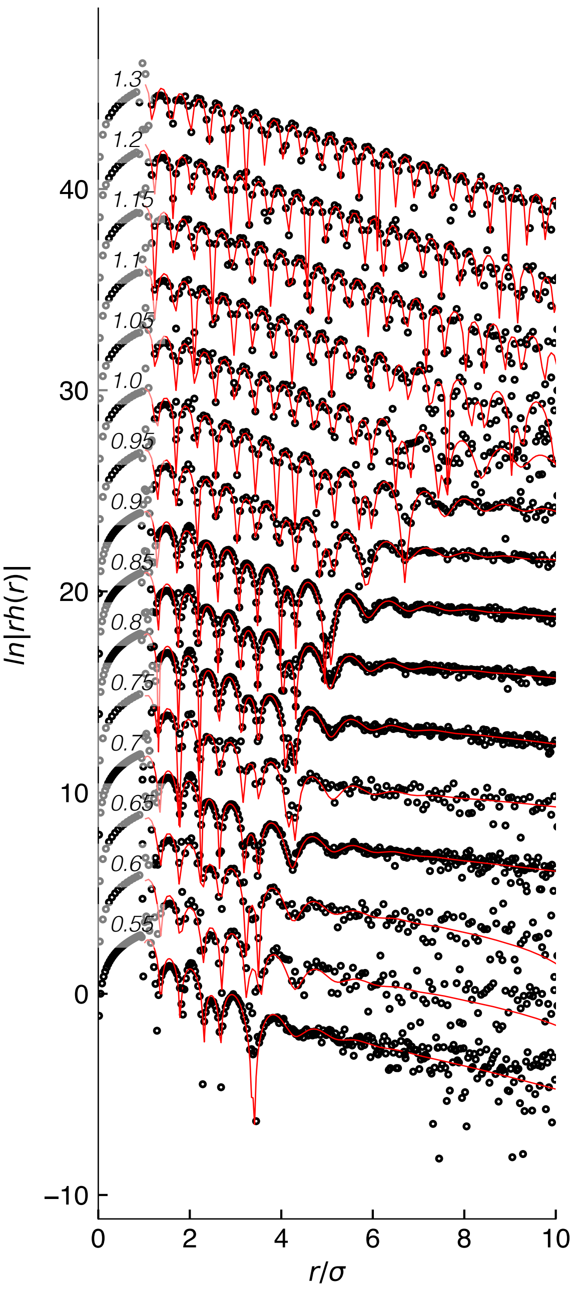


FIG. S6. Scaled total correlation functions at Pe = 28 for a range of densities (black) fitted by Eq. 9 (red).

## S4. FORM OF THE EFFECTIVE TWO-BODY POTENTIAL

The effective two-body potential emerging from the active dynamics cannot be trivially rescaled at different Péclet numbers. To show this, we plot in Fig. S8 the potential rescaled by its minimum. This corresponds to a rescaling by the interaction

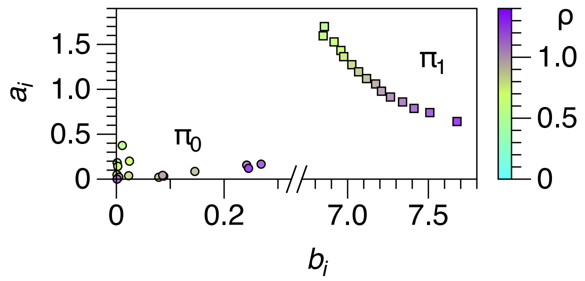


FIG. S7. Two poles $\pi_1$ and $\pi_2$ and their respective lengthscales with increasing number density at Pe = 28.

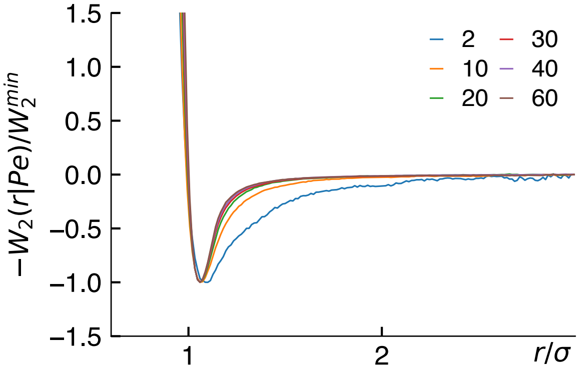


FIG. S8. Effective twobody potential for the 3D ABPs for different values of the Péclet number, rescaled by the well depth $W_2^{\min}$.

strength in depletion potential such as the single species, Asakura-Oosawa model [10].

We find that the attractive well of the potential varies rapidly from the low Pe to the near critical Pe regime. The attractive branch converges to zero slowly for small Pe and gradually more rapidly as we reach near-critical values of the Péclet number. As we increase Pe, the well becomes narrower.

Numerical evidence suggests that the effective potential converges to a master curve at very high Pe. We interpret this as the convergence to a regime where the orientation of the self-propulsion no longer relaxes and where only the elastic collisions between the particles contribute to their re-orientation.

## S5. TWO-DIMENSIONAL TEST OF VLIEGENTHART-LEKKERKERKER'S CRITERION

A key insight of our work is that effective 2-body interactions do not engender phase separation. We rationalise this fact by employing ideas derived from the theory of simple liquids. Specifically it is known that the second virial coefficient $B_2$ provides a approximate criterion for locating criticality in simple liquids. This observation - originally made in 3D by Vliegenthart and Lekkerkerker - can be generalised to other dimensions [11] and implies that near criticality

$$B_2(T)/\nu_0 \approx -C \tag{10}$$

$$B_2(T) = -\frac{1}{2}\int (e^{-V(r)/k_BT} - 1)d\boldsymbol{r} \tag{11}$$

with $C$ a dimensionality-dependent constant, $V(r)$ the interaction potential and $\nu_0$ is the (effective) hard-sphere volume in d-dimensions, here approximated by $\nu_0 = \pi^{d/2}(\sigma/2)^d/\Gamma(d/2+1)$. While Vliegenthart and Lekkerkerker focussed on 3D systems, obtaining $C \approx 6$ for the reference value for 2D systems one finds from previous studies of criticality in the 2d Lennard-Jones fluids [12] that $B_2(T_c)/\nu_0 = -8.2$.

In the work reported in the manuscript, instead of the interaction potential $V(r)/k_BT$ we employ, for every Péclet number, the effective two-body interaction $W(r|Pe)$ extracted from the simulations of $N = 2$ ABPs. We find that for the 3d case the effective $B_2$ never crosses the Vliegenthart-Lekkerkerker criterion, hence a passive model with pair interactions extracted from the active systems does not phase separate.

The same is true for the 2d system. To do so, we follow Stenhammar et al. [1] and consider the two dimensional version of Eq. 2,3, with the same repulsive interactions and Péclet number as the 3d system.

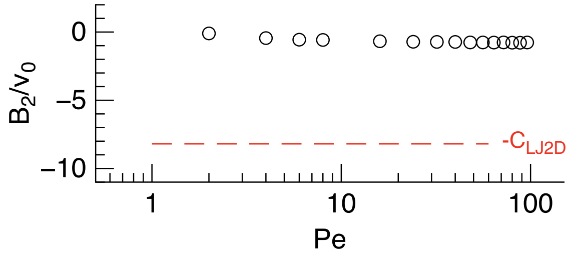


FIG. S9. Reduced effective second virial coefficient for two-dimensional ABPs.

In Fig. S9 we plot the effective reduced $B_2$ and compare it with the approximate Vligenhardt-Lekkerkerker criterion: $B_2(T_c)/\nu_0 = -8.2$. As the plot shows, the measured values of $B_2$ remain far apart over the entire range of Péclet numbers, including the region for which it is known MIPS occurs in ABPs (about Pe = 30 − 40). This indicates

that no phase separation occurs in the 2-body passive model and that the conclusions that we have drawn for 3d apply to the 2d case too.

## S6. EQUILIBRIUM SIMULATIONS AND SMALL BOX MULTIBODY PROBABILITIES

In order to assess the emergence of multibody effects in the active dynamics, we compare the steady-state statistics from active Brownian particles simulations to equilibrium (passive) Monte-Carlo simulations with effective twobody interactions, extracted as described in the main text.

The Monte-Carlo simulations reflect the geometries of the active system: for example, when we probe the possibility of phase separation at high $Pe$, we consider the same slab geometry as the active system (same box size and number of particles), with initialised dense and less dense phases.

The equilibrium algorithm is a standard local Monte-Carlo scheme, whereby particles attempt displacements whose components have a maximal value of $0.2\sigma$ with an effective twobody interaction $U(r;\mathrm{Pe}) = W_2(r;\mathrm{Pe})/\beta$ . We take the inverse temperature scale to be $\beta = 1$ and for every reference Pe we take the corresponding effective twobody potential.

For the calculation of the $P^N(r_{\min})$ probabilities for the active and twobody passive systems we again consider identical geometries for the two different dynamics. We consider cubic boxes of linear size $L = 8.7\sigma$. This value is chosen as it allows to accommodate 6 particles of size $\sigma$ on the main diagonal, meaning that for $N \leq 6$ we are able to sample non-interacting conditions. For larger $N$ the probability of non-interacting configurations is rapidly decreasing with $N$. Since for the active system it is not possible to implement biasing techniques in the absence of a free energy, we perform brute force calculations of the probability distributions: we take $\sim 10^4$ independent random initial configurations and run trajectories of duration $1000\tau_r$. For the passive system, a standard local Monte-Carlo sampling is performed. Through subsampling, we monitor the errorbars on the probability distributions $P^N(r_{\min})$ and arrest the equilibrium sampling when we reach the same degree of accuracy of the active Brownian particle sampling.

TABLE S1. Summary of the system sizes employed to study finite size effects.

| | Gas-Solid | MIPS |
|---|---|---|
| Lx | $131\sigma$ | $143\sigma$ |
| Ly | $[23, 113]\sigma$ | $[25, 127]\sigma$ |
| N | $[85, 2126] \cdot 10^3$ | $[70, 1728] \cdot 10^3$ |

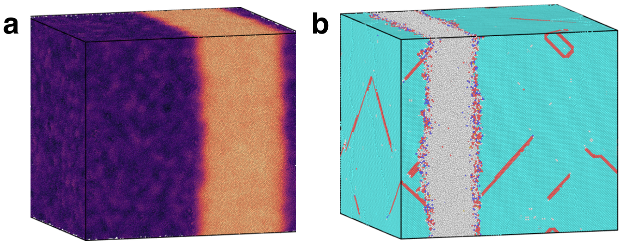


FIG. S10. Snapshots from large scale simulations of (a) the coexisting MIPS phase and (b) the coexisting gas-crystal at Pe = 70. In (a), particles are colour-coded according to their local coordination withing $2\sigma$, in the range 11−170. In (b), particles are color-coded according to their FCC (cyan), or HCP (red), or BCC (blue) local environment.

## S7. FINITE-SIZE EFFECTS IN THE COEXISTENCE DENSITIES

As we approach the high Pe region, the active systems develop an increasing persistence length, defined as

$$\ell_p = \sigma \mathrm{Pe}. \tag{12}$$

As the critical point of the three-dimensional ABPs is around Pe $\approx 40$, very large system sizes are required in order to limit the finite-size effects in the MIPS and gas-crystal phase separation.

To test the robustness of our estimates of the coexistence densities, we performed large-scale simulations in the slab geometry, both for the gas-solid and the motility-induced phase at a representative Péclet number Pe = 70, where $\ell_p = 70\sigma$. As illustrated in Table S1 these allow us to explore lengths up to about $2\ell_p$ and involve, for the largest systems here considered, more than 2 100 000 particles.

We estimate the coexistence densities from the lateral density profile along the $x$ dimension, evaluated at steady state (i.e. after $200\tau_r$) form 20 independent configurations, see Fig S10 for representative snapshots. In Fig. S11 we observe that there are some systematic finite size effects in the measured densities. However, these are small (deviations below 1%) both for MIPS and the gas-solid coexistence. This demonstrates that results are robust

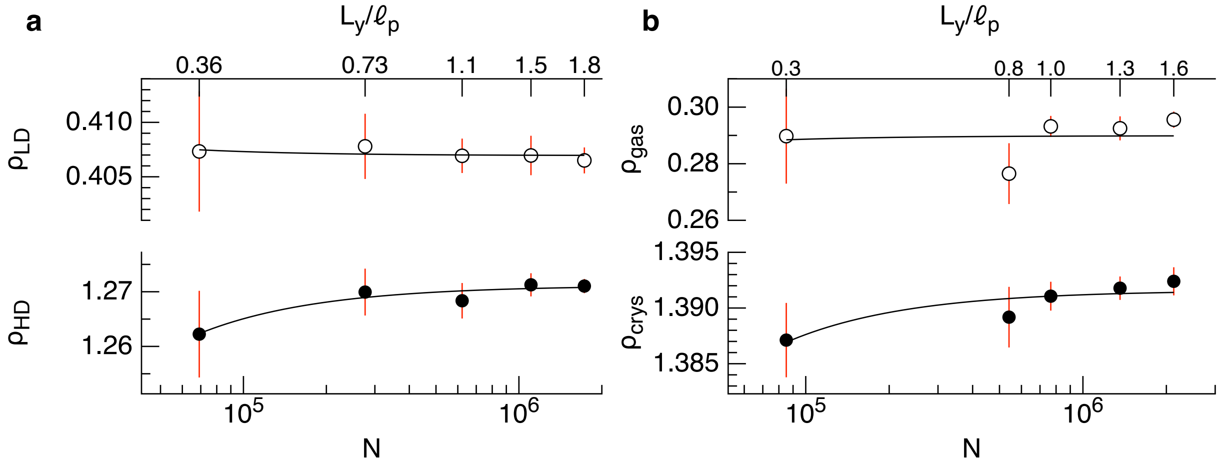


FIG. S11. Finite size effects in the determination of the coexistence densities for (a) MIPS and (b) gas-crystal coexistence. Vertical red bars are standard deviations from samples of 20 independent configurations at steady state. Continuous lines are guides to the eye.

with respect to finite size effects. We note that, as it is the case for equilibrium phase diagrams, the region around he critical point may be more severely affected by finite-size effects, whose specific study goes beyond the scope of the present work.

## S8. N-BODY CORRELATIONS AND $P_N(\mathrm{r}_{\min})$

Here we briefly summarise the formalism developed in [13]. Consider a simulation box of volume $V$ containing a small fixed number $N$ of interacting particles. At thermal equilibrium, the probability of a configuration is

$$P_N\left(\mathbf{r}^N\right) = \frac{e^{-\beta U\left(\mathbf{r}^N\right)}}{Z_N}, \tag{13}$$

with $\boldsymbol{r}^N$ is the vector of particle positions, $\beta = 1/(k_B T)$ is the inverse temperature, $U(\boldsymbol{r}^N)$ is the interaction potential, and $Z_N$ is the (configurational) partition function

$$Z_N = \int e^{-\beta U\left(\mathbf{r}^N\right)} \mathrm{d}\mathbf{r}^N. \tag{14}$$

Let us define

$$\tilde{g}_N\left(\mathbf{r}^N\right) \equiv \frac{P_N\left(\mathbf{r}^N\right)}{P_N^{\mathrm{ig}}\left(\mathbf{r}^N\right)} = V^N \frac{e^{-\beta U\left(\mathbf{r}^N\right)}}{Z_N}, \tag{15}$$

with $P_N^{\mathrm{ig}}\left(\mathbf{r}^N\right) = V^{-N}$ is the probability of finding $N$ ideal gas particles in same configuration as the selected particles. In the limit when the particles are not interacting (i.e. the are separated by a distance larger than the interaction range $R$) we define the asymptotic value

$$f_N(V) \equiv \tilde{g}_N\left(\mathbf{r}^N\right) \quad |\mathbf{r}_k - \mathbf{r}_l| > R, \forall k, l \tag{16}$$

$$= \frac{Z_1}{Z_N}. \tag{17}$$

Then the excess free energy $F_{ex}(N)$ follows as

$$F_{ex}(N) = -k_B T \ln f_N. \tag{18}$$

Although it has the low density limiting behaviour $\lim_{V\to\infty} f_N(V) = 1$, (because $Z_N$ is dominated by configurations in which the N particles are well separated) for finite system volume $f_N(V)$ deviates from unity.

While Eq. 16 would require populating with high accuracy a $3N$-dimensional histogram, it is possible to simplify the expression. To do so, we consider

$$g_N'\left(r_{\min}\right) \equiv \frac{P_N\left(r_{\min}\right)}{P_N^{\mathrm{ig}}\left(r_{\min}\right)}, \tag{19}$$

where $r_{\min}$ is the shortest distance between the $N$ particles.

The non-interacting regime for which $|\mathbf{r}_k - \mathbf{r}_l| > R, \forall k, l$ is identical to the limit of large $r_{\min}$. In this limit one has that the probability $P_N(\boldsymbol{r}^N) = Z_N^{-1}$ while the ideal gas probability is $V^{-N}$. It follows that the asymptotic value of $g_N'\left(r_{\min}\right)$ is equal to the asymptotic value of $\tilde{g}_N\left(\mathbf{r}^N\right)$, i.e.

$$g'_N\left(r_{\min} > R\right) = f_N(V), \tag{20}$$

which provides a viable computational route to evaluate the $f_N(v)$.

Operationally, one can therefore estimate the $f_N(V)$ from the shortest distance probabilities as

$$f_N(V) = \frac{\int_{r_l}^{r_u} P_N\left(r_{\min}\right) \mathrm{d}r_{\min}}{\int_{r_l}^{r_u} P_N^{\mathrm{ig}}\left(r_{\min}\right) \mathrm{d}r_{\min}}, \tag{21}$$

where $r_l, r_u$ and lower and upper bounds for the integration which take into account the requirement to attain the asymptotic limit and to maximise the signal to noise ratio.

In the context of equilibrium systems, virial coefficents of increasing order can be expressed in terms of the $f_N(V)$ [13]. However, the expression in Eq. 21 can be easily computed also in the non-equilibrium case of active particles and it acts as a structural measure of the emerging many-body correlations, as discussed in the main text.


[1] J. Stenhammar, D. Marenduzzo, R. J. Allen, and M. E. Cates, Soft Matter **10**, 1489 (2014).

[2] S. Das, G. Gompper, and R. G. Winkler, New Journal of Physics **20**, 015001 (2018).

[3] S. Plimpton, Journal of computational physics **117**, 1 (1995).

[4] C. Bechinger, R. Di Leonardo, H. Löwen, C. Reichhardt, G. Volpe, and G. Volpe, Reviews of Modern Physics **88** (2016).

[5] M. Rovere, D. W. Hermann, and K. Binder, Europhysics Letters (EPL) **6**, 585 (1988).

[6] J.-P. Hansen and I. R. McDonald, *Theory of simple liquids: with applications to soft matter* (Academic Press, 2013).

[7] D. Villamaina and E. Trizac, European Journal of Physics **35**, 035011 (2014).

[8] A. Statt, R. Pinchaipat, F. Turci, R. Evans, and C. P. Royall, Journal of Chemical Physics **144** (2016).

[9] D. Stopper, H. Hansen-Goos, R. Roth, and R. Evans, The Journal of chemical physics **151**, 014501 (2019).

[10] K. Binder, P. Virnau, and A. Statt, J Chem Phys **141**, 140901 (2014).

[11] V. L. Kulinskii, The Journal of chemical physics **134**, 144111 (2011).

[12] Y. Liu, A. Z. Panagiotopoulos, and P. G. Debenedetti, The Journal of chemical physics **132**, 144107 (2010).

[13] D. J. Ashton and N. B. Wilding, The Journal of chemical physics **140**, 244118 (2014).
